# Supplementary material for: Deep Semi-supervised Knowledge Distillation for Overlapping Cervical Cell Instance Segmentation
Source: arXiv:2007.10787 ancillary file (2020-07-21)
Supplement: Supplementary file 1 [file supplementary.pdf]

# — Supplementary Material —
# Deep Semi-supervised Knowledge Distillation for Overlapping Cervical Cell Instance Segmentation

Yanning Zhou[1], Hao Chen[1], Huangjing Lin[1], Pheng-Ann Heng[1,2]

[1]Department of Computer Science and Engineering, The Chinese University of Hong Kong, Hong Kong SAR, China
{ynzhou,hchen,hjlin,pheng}@cse.cuhk.edu.hk
[2]Guangdong Provincial Key Laboratory of Computer Vision and Virtual Reality Technology, Shenzhen Institutes of Advanced Technology, Chinese Academy of Sciences, Shenzhen, China

## 1 Details of Augmentation

| Augmentation | Description | Parameter | Value |
|---|---|---|---|
| Brightness | Adjusts the brightness of the image. $B = 0$ gives a black image, $B = 2$ increases the brightness by a factor of 2. | $B$ | $[0.85, 1.15]$ |
| Contrast | Adjusts the contrast of the image. $C = 0$ gives a solid gray image, $C = 2$ increases the contrast by a factor of 2. | $C$ | $[0.85, 1.15]$ |
| Hue | The image hue is adjusted by converting the image to HSV and cyclically shifting the intensities in the H channel by the factor $H$. | $H$ | $[0.95, 1.05]$ |
| Erasing | Randomly selects a rectangle region in a image and erases its pixels with random values. The notations of hyper-parameters are same as those described in [1]. | $p$<br>$s_l$<br>$s_h$<br>$r_1$<br>$r_2$ | $p = 0.7$<br>$s_l = 0.001$<br>$s_r = 0.004$<br>$r_1 = 0.2$<br>$r_2 = 5$ |
| Flip | Flips the image along the vertical or horizontal axis with a probability of $p$. | $p$ | 0.5 |

Table 1: List of augmentations along with their corresponding parameters used in both the student network and the teacher network.

Table 1 shows the details of augmentation methods which are used in both the student network and the teacher network. Specifically, each time we double the transformed images by adding a flipped version for the teacher network.

## 2 Pseudo Code for the Proposed Framework

---

**Algorithm 1** Mask-guided Mean Teacher with Perturbation-sensitive Sample Mining (MMT-PSM) Training Strategy

---

**Require:** Labeled data $\mathcal{D}_L$, unlabeled data $\mathcal{D}_U$, teacher augmented time $K$ and student augmented time $L$
**Require:** Negative sample number $s$, ensembling momentum $\alpha$, weight function $\lambda(t)$
**Require:** Student $S$ with weight $\theta$ and teacher $T$ with weight $\theta'$
**for** $t$ in $[1, 1000]$ **do**
    $\{x_i^l, y_i^l\} \leftarrow \mathit{Sample}(\mathcal{D}_L)$
    Optimize the student network via the supervised loss $\mathcal{L}_{sup}\left(S\left(x_i^l\right), y_i^l\right)$
**end for**
Initialize the teacher network $\theta'_t \leftarrow \theta_{t-1}$
**for** $t$ in $[1000, \mathit{num\_iterations}]$ **do**
    $\{x_i^l, y_i^l\} \leftarrow \mathit{Sample}(\mathcal{D}_L)$, $\{x_i^u\} \leftarrow \mathit{Sample}(\mathcal{D}_U)$
    Calculate the supervised loss $\mathcal{L}_{sup}\left(S\left(x_i^l\right), y_i^l\right)$
    Generate augmented samples $\{x_{i,1}^{\mathcal{T}}, \ldots, x_{i,K}^{\mathcal{T}}\} \leftarrow \mathit{Augmentor}(x_i^u)$ for $T$ and $\{x_{i,1}^{\mathcal{S}}, \ldots, x_{i,L}^{\mathcal{S}}\} \leftarrow \mathit{Augmentor}(x_i^u)$ for $S$
    `/* for teacher network */`
    Feed $\{x_{i,1}^{\mathcal{T}}, \ldots, x_{i,K}^{\mathcal{T}}\}$ to $T$
    Get proposals $\mathcal{R}_{x_i^{\mathcal{T}}}$ from RPN and features $Z^{\mathcal{T}}$
    Calculate the average soft pseudo labels $\bar{P}_i$ by equation 1 and the variance of predictions by equation 2
    Preserve $\bar{P}_i$ for all positive samples and top $s$ negative samples
    Generate segmentation mask $M$ via integrating instance mask predictions
    `/* for student network */`
    Feed $\{x_{i,1}^{\mathcal{S}}, \ldots, x_{i,L}^{\mathcal{S}}\}$ to $S$
    Set teacher's proposals to student $\mathcal{R}_{x_i^{\mathcal{S}}} = \mathcal{R}_{x_i^{\mathcal{T}}}$
    Calculate the perturbation-sensitive sample mining loss $\mathcal{L}_{psm}$ by equation 3 and mask-guided distillation loss $\mathcal{L}_{mgd}$ by equation 4
    `/* weight update */`
    Calculate the overall objective function by equation 5 and optimize the student's parameters $\theta$ via gradient descent
    Update temporally average teacher model $\theta'_t \leftarrow \alpha\theta'_{t-1} + (1-\alpha)\theta_{t-1}$
**end for**

---

Algorithm 1 summaries the proposed MMT-PSM framework. Noticed that whenever a geometric transformation is conducted during augmentation, the predictions perform the reverse transformation on their locations before calculating the average soft pseudo labels to keep the label space consistent. In addition, since the foreground/background-balanced sampling strategy is used to select training samples for RPN and Box Head in the Mask R-CNN [2]. We randomly choose one augmented sample in teacher network to generate the coarse predictions for training sample selection.

## 3 Parameter Analysis

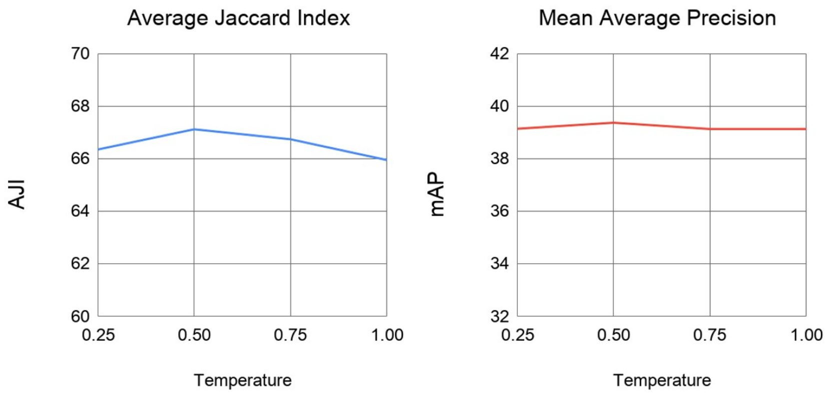


Fig. 1: Performance evaluation of our proposed MMT-PSM with different values of temperature $t$, which determines the sharpness of the ensemble pseudo labels.

A sharpen function $S(\overline{P}_i) = \overline{P}_i^t / \sum_{j=1}^{c} \overline{P}_j^t$ is further used to implicitly achieve entropy minimization [3], in which $c$ denotes the number of categories. When $t \rightarrow 0$, the output will approach a Dirac distribution, which encourages the model to produce lower-entropy prediction. When $t = 1$, the output is identical to the input. We conducts experiments with different temperatures and find $t = 0.5$ as the optimal value in our study.

## References

1. Zhong, Z., Zheng, L., Kang, G., Li, S., Yang, Y.: Random Erasing Data Augmentation. In: AAAI. pp. 13001-13008 (2020)
2. Girshick, R., Randosavovic, I., Gkioxari, G., Dollár, P., He, K.: Detectron. https://github.com/facebookresearch/detectron (2018)
3. Berthelot, D., Carlini, N., Goodfellow, I., Papernot, N., Oliver, A., Raffel, C.A.: Mixmatch: A holistic approach to semi-supervised learning. In NeurIPS. pp. 5050-5060 (2019)
